# Supplementary material for: Ensembles of Multiple Models and Architectures for Robust Brain Tumour Segmentation
Source: arXiv:1711.01468 source file (2017-11-04)
Supplement: Supplementary file 1 [file appendix.tex]

% !TeX root=../paper.tex

\section{Appendix}
\label{sec:appendix}

\begin{table}[htbp]
  \caption{Architectures for FCN-VGG and FCN-ResNet. The first two columns list the resolution scale and feature map size. The third and fourth columns list the convolutional layer parameters for the two architectures, with ``$3 \times 3 \times 3, 16$" denoting 3$\times$3$\times$3 kernel and 16 output features. For FCN-ResNet, the residual blocks are shown in brackets, with the number of blocks stacked. \label{tab:FCN}}
  \centering
  \begin{tabular}{c|c|c|c}
  \hline 
  scale & size & FCN-VGG & FCN-ResNet \\
  \hline 
  1 & 64$\times$64$\times$64 & $\begin{array}{c}3 \times 3 \times 3, 16\\ 3 \times 3 \times 3, 16\end{array}$ \\
  \hline
  2 & 32$\times$32$\times$32 & $\begin{array}{c}3 \times 3 \times 3, 32\\ 3 \times 3 \times 3, 32\end{array}$  \\
  \hline
  3 & 16$\times$16$\times$16 & $\begin{array}{c}3 \times 3 \times 3, 64\\ 3 \times 3 \times 3, 64\\ 3 \times 3 \times 3, 64\end{array}$ & normal building block\red{?} $\left[\begin{array}{cc}3 \times 3 \times 3, 64\\ 3 \times 3 \times 3, 64\end{array}\right] \times 4$ \\
  \hline
  4 & 8$\times$8$\times$8 & $\begin{array}{c}3 \times 3 \times 3, 128\\ 3 \times 3 \times 3, 128\\ 3 \times 3 \times 3, 128\end{array}$ & bottleneck building block\red{?} $\left[\begin{array}{cc}1 \times 1 \times 1, 128\\ 3 \times 3 \times 3, 128\\ 1 \times 1 \times 1, 512\end{array}\right] \times 4$ \\
  \hline
  5 & 4$\times$4$\times$4 & $\begin{array}{c}3 \times 3 \times 3, 256\\ 3 \times 3 \times 3, 256\\ 3 \times 3 \times 3, 256\end{array}$ \\
  \hline
  \multicolumn{4}{c}{upsample and concatenate} \\
  \multicolumn{4}{c}{scale 1 to 5 features} \\
  \hline
  predict & 64$\times$64$\times$64 & $\begin{array}{c}1 \times 1 \times 1, 64\\ 1 \times 1 \times 1, 64\\ 1 \times 1 \times 1, K\end{array}$ \\
  \hline
  \end{tabular} 
\end{table}

% Please add the following required packages to your document preamble:
% \usepackage[table,xcdraw]{xcolor}
% If you use beamer only pass "xcolor=table" option, i.e. \documentclass[xcolor=table]{beamer}
\begin{table}[]
\label{table:UNet}
\caption{U-Net architecture}
\centering
\begin{tabular}{|
>{\columncolor[HTML]{EFEFEF}}c |c|c|c|c|c|c|}
\hline
\textbf{Layer Type} & \cellcolor[HTML]{EFEFEF}\textbf{\# Output Filters} & \cellcolor[HTML]{EFEFEF}\textbf{Kernel Size} & \cellcolor[HTML]{EFEFEF}\textbf{Stride} & \cellcolor[HTML]{EFEFEF}\textbf{Dropout ratio} & \cellcolor[HTML]{EFEFEF}\textbf{BatchNorm} & \multicolumn{1}{l|}{\cellcolor[HTML]{EFEFEF}\textbf{Non-linearity}} \\ \hline
Conv & 16 & 3 & 1 & - & Yes & ReLU \\ \hline
Conv & 16 & 3 & 1 & - & Yes & ReLU \\ \hline
Max-pooling & - & 2 & 2 & - & - &  \\ \hline
Conv & 32 & 3 & 1 & - & Yes & ReLU \\ \hline
Conv & 32 & 3 & 1 & - & Yes & ReLU \\ \hline
Max-pooling & - & 2 & 2 & - & - &  \\ \hline
Conv & 64 & 3 & 1 & - & Yes & ReLU \\ \hline
Conv & 64 & 3 & 1 & - & Yes & ReLU \\ \hline
Max-pooling & - & 2 & 2 & - & - & - \\ \hline
Conv & 128 & 3 & 1 & - & Yes & ReLU \\ \hline
Conv & 128 & 3 & 1 & 0.5 & Yes & ReLU \\ \hline
Upsampling & \multicolumn{6}{c|}{x 2 using repetition} \\ \hline
Conv & 64 & 3 & 1 & - & Yes & ReLU \\ \hline
Conv & 64 & 3 & 1 & 0.5 & Yes & ReLU \\ \hline
Upsampling & \multicolumn{6}{c|}{x 2 using repetition} \\ \hline
Conv & 32 & 3 & 1 & - & Yes & ReLU \\ \hline
Conv & 32 & 3 & 1 & 0.5 & Yes & ReLU \\ \hline
Upsampling & \multicolumn{6}{c|}{x 2 using repetition} \\ \hline
Conv & 16 & 3 & 1 & - & Yes & ReLU \\ \hline
Conv & 16 & 3 & 1 & - & Yes & ReLU \\ \hline
Conv & \#labels & 3 & 1 & - & - & Softmax \\ \hline
\end{tabular}
\end{table}
